# Supplementary material for: Refinements of chromatic towers and Krull-Schmidt decompositions in stable homotopy categories
Source: arXiv:math/0607726 source file (2006-07-28)
Supplement: Supplementary file 1 [file appendix.tex]

%
% Appendix
%

\chapter{Two out of three subcategories}

Recall that an analogue for a thick subcategory of $D(R)$ in the category of $R$-modules is the so called Wide subcategory
-- an abelian category that is closed under extensions. Now we ask for a similar analogy 
for triangulated subcategories, i.e, what is the right analogue of a triangulated subcategory in the
world of modules? Towards this, we propose the following definition.

\begin{defn} A subcategory $\C$ of an abelian subcategory $\mathscr{A}$ is said to be a  2-3\emph{ (two out of three) subcategory} 
if whenever 
\[0 \rar A \rar B \rar C \rar 0\] 
is a s.e.s in $\mathscr{A}$ such that two out of the three objects appearing in the
short exact sequence belong to $\C$, then so does the third object.
\end{defn}

It is clear from this definition that every wide subcategory of $\mathscr{A}$ is also a 2-3 subcategory. Here is an example of 
a 2-3 subcategory that is not wide.

\begin{example} The subcategory $\C$ of all even dimensional rational vector spaces in the category $\mathscr{A}$ of finite dimensional rational
vector spaces is readily seen to be a 2-3 subcategory. However, this is not a wide subcategory: Consider the projection map
\[
\begin{array}{ccc}
\mathbb{Q}^2 & \longrightarrow &  \mathbb{Q}^2 \\
(x,y) &  \longmapsto  & (x,0). 
\end{array}
\]
This map has a one (odd) dimensional kernel and hence the subcategory $\C$ is not closed under kernels and therefore not wide.
\end{example}

We now classify all the 2-3 subcategories in the category $\mathscr{A}$ of finitely generated modules over a 
PID.  We first set up some notations. Through out this appendix $R$ will denote a principal ideal domain (PID). 
For every prime ideal $p$ in $R$, define an Euler characteristic function $\chi_p$ on $\mathscr{A}$ as follows:
\[ 
\chi_p(X) :=
 \left\{
   \begin{array}{ll}
      \length (X \otimes_R R_{(p)}) & \mbox{ when $p \ne 0$} \\
      \dim_{R_{0}}( X \otimes_R R_{0})  & \mbox{ when $p =0$}
    \end{array}
 \right. 
\]

These Euler characteristic functions will define some full subcategories of $\mathscr{A}$:
For each non-negative integer $k$, define $I_k$ as
\[ I_k = \{ X \in \mathscr{A}: \chi_0(X) \equiv 0\mod k \}, \]
and for a given subset $S$ of non-zero primes in $Spec(R)$ and a subgroup $H$ of ${\underset{p \in S}{\oplus}}\mathbb{Z}$, define $F(S,H)$ as 
\[F(S,H) = \{ X \in \mathscr{A}: {\underset{p \in S}{\oplus}}  \chi_p(X) \in H\}. \]
Note that since $\chi_p$ is an Euler characteristic function, all these subcategories are 2-3 subcategories. We now show that these
are all the 2-3 subcategories in $\mathscr{A}$. 

\begin{prop} Let $R$ be a PID and let $\mathscr{A}$ denote the category of finitely generated $R$-modules.
Then a subcategory $\C$ is a 2-3 subcategory if and only if either $\C = I_k$ for some integer $k$, or $\C= F(S,H)$
for some subset $S$ of $Spec(R)$ and a subgroup $H$ of $\underset{p \in S}{\oplus} \mathbb{Z}.$
\end{prop}

\begin{proof}  The only tool that we use here is the structure theorem for finitely generated modules over a PID!.
Let $\C$ be a 2-3 subcategory of $\mathscr{A}$. The proof divides naturally into two cases.

Case(i) \emph{$\C$ contains a module of rank at least one.} Pick a module, $M$ say, of smallest non-zero rank
(exists by assumption) and let $k$ denote the rank of $M$. We claim that $\C = I_k$. In other words, we have to show that 
$\C$ comprises of all modules of the form $R^{kl} \oplus T$ where $l$ is a non-negative integer and $T$ is a torsion module. 
This will be done by following a series of straight forward reductions.  First of all, it suffices
to build $R^k$, and any given torsion module, starting from $M$ (because 2-3 subcategories are closed under taking direct sums). Then, the 
exact sequence
\[ 0 \rar Tor(M) \rar M(= R^k \oplus Tor(M)) \rar R^k \rar 0\]
gives a further reduction: It suffices to build an arbitrary torsion module out of $M$. Now recall from the structure theorem that any 
torsion module is a direct sum of cyclic modules of the form $R/p^t$. Again, 2-3 subcategories are closed under taking direct sums,
therefore it is enough to produce $R/p^t$ for any prime $p$ and any integer $t$. The following short exact sequence tells us that this is
always possible: (here we use the fact that $k\ge1$)
\[ 0 \rar R \oplus( R^{k-1} \oplus Tor{M} ) \;\; {\overset{p^k \oplus id}{\longrightarrow}} \;\; R \oplus (R^{k-1} \oplus Tor{M})  
\rar R/p^t \rar 0.\]
So this completes the first case.

Case(ii) \emph{All modules in $\C$ have rank zero.}  This means that $\C$ consists of torsion modules. For simplicity, we will assume 
that $\C$ consists of modules that have only $p$-torsion, for a fixed prime $p$. The general case is similar but only more cumbersome to write down.
With this assumption, pick a non-zero module $M$ of smallest $p$-length, $l$ say. Then by the structure theorem, 
$M \cong \oplus_{i=1}^{k} R/p^{r_i}$ with $\sum r_i = l$.
We will show that $\C=F(p,l\mathbb{Z})$.  This will be done in two steps. The first step shows that we can generate
$\oplus_{i=1}^{l} R/p$. The second shows that we can generate any module in $F(p,l\mathbb{Z})$ using $\oplus_{i=1}^{l} R/p$. 
Clearly these two steps will imply the claim. 

Step 1. The idea is to start with $\oplus_{i=1}^{k} R/p^{r_i}$, and generate modules with lower highest order 
(In the module $\oplus_{i=1}^{k} R/p^{r_i}$, the
highest order is $max\{r_i\}$.) until we get a module with highest order $=1$, or equivalently, until we get $\oplus_{i=1}^{l} R/p$.
Again for better clarity of the proof, we break this into parts.

(a) First we build $R/p \oplus R/p^{r_1-1}$ from $R/p^{r_1}$. The following pair of short exact sequences will do this.
(The maps are easy to guess, so we will not bother to write them down.)
\[ 0 \rar R/p^{r_1} \rar R/p^{r_1-1} \oplus R/p^{r_1+1} \rar R/p^r_1 \rar 0\]
\[ 0 \rar R/p^{r_1} \rar R/p^{r_1-1} \oplus R/p^{r_1+1} \rar R/p^{r_1-1} \oplus R/p  \rar 0\]

(b) Now we build $R/p \oplus R/p^{r_1-1} \oplus R/p^{r_2} \oplus \cdots \oplus R/p^{r_k}$ from 
$R/p^{r_1} \oplus R/p^{r_2} \oplus \cdots \oplus R/p^{r_k}$. (Note that this decreases the highest order by one.)
This can be obtained easily by adding a $G= \oplus_{i=2}^{k} R/p^i$
to the above pair of short exact sequences as follows.
\[ 0 \rar R/p^{r_1} \oplus G \rar (R/p^{r_1-1} \oplus G) \oplus (R/p^{r_1+1} \oplus G)\rar R/p^{r_1} \oplus G \rar 0\]
\[ 0 \rar R/p^{r_1} \oplus G \rar (R/p^{r_1-1} \oplus G) \oplus (R/p^{r_1+1} \oplus G)\rar R/p^{r_1-1} \oplus R/p \oplus G \rar 0\]

(c) A straight forward downward induction will decrease the highest order to $1$. In other words, it produces
$\oplus_{i=1}^{l} R/p$, completing the proof of step 1.

Step 2. Starting with $\oplus_{i=1}^{l} R/p$, we want to build any module in $\C_l$, i.e., any $2$-torsion module of 
length $lx$, where $x$ is any non-negative integer. Towards this, we make another reduction. It is enough to generate any module of
length $l$: Since 2-3 subcategories of closed under taking direct sums, $\C$ also has $(\oplus_{i=1}^{l} R/p)^x$, and so 
the same construction that generates a module of length $l$ from $\oplus_{i=1}^{n} R/p$, will work in the general case.

Recall that an arbitrary module of length $l$ looks like $\oplus R/p^{r_i}$, with $\sum r_i = l$. So we have to
start with $\oplus_{i=1}^{l} R/p$ and construct the module  $\oplus R/p^{r_i}$. Again for clarity, we break the construction into parts..

(a) We first generate $R/p^{r+1}$ from $R/p^r \oplus R/p$. The following pair of short exact sequences will do this job.
\[ 0 \rar R/p \oplus R/p^r \rar R/p \oplus R/p^{r+1} \oplus R/p^{r} \rar R/p \oplus R/p^r \rar 0\] 
\[ 0 \rar R/p \oplus R/p^r \rar R/p \oplus R/p^{r+1} \oplus R/p^{r} \rar \oplus R/p^{r+1} \rar 0\] 

(b) Now we generate $R/p^{r+1} \oplus G$ from $R/p^r \oplus R/p \oplus G$. ($G$ is an arbitrary $p$-torsion module.)
\[ 0 \rar R/p \oplus R/p^r \oplus G \rar R/p \oplus R/p^{r+1} \oplus R/p^{r} \oplus G \oplus G \rar R/p \oplus R/p^r \oplus G\rar 0\] 
\[ 0 \rar R/p \oplus R/p^r \oplus G \rar R/p \oplus R/p^{r+1} \oplus R/p^{r} \oplus G \oplus G \rar R/p^{r+1} \oplus G\rar 0\] 

(c) Now, as before, a simple induction will tell us that given any partition(unordered) of $l$ as $l=\sum r_i$, we can generate $\oplus R/p^{r_i}$
starting from $\oplus_{i=1}^{l} R/p$.
This completes step 2 and therefore the proof of the proposition.
\end{proof}

\begin{rem} The proposition is a result of our attempt towards establishing a correspondence between subgroups of the Grothendieck
groups of a wide subcategory and some sort of ``triangulated subcategories of modules''.  Our hope was that the 2-3 subcategories will be the
right candidates for these ``triangulated subcategories 
of modules''. Recall that if $R$ is a PID, that the Grothendieck group of the wide subcategory $W_S$, corresponding to a set $S$ of non-zero primes 
in $R$, is ${\underset{p \in S}{\oplus}}\mathbb{Z}$. (Note that this wide subcategory is just the collection of all finitely generated torsion 
modules with torsion contained in $S$.) It is clear now, from the proof of the above proposition, that the 2-3 subcategories of $W_S$
are in bijection with the subgroups of the Grothendieck group $K_0(W_S)$!. However, this correspondence fails when $S =Spec(R)$. 

\end{rem}
